# Supplementary material for: Symphonize 3D Semantic Scene Completion with Contextual Instance Queries
Source: arXiv:2306.15670 source file (2023-11-22)
Supplement: Supplementary file 1 [file X_suppl.tex]

\clearpage
\setcounter{page}{1}

\renewcommand{\maketitlesupplementary}{
    \newpage{
       % \twocolumn[
        \onecolumn
        \centering
        \Large
        \textbf{\thetitle} \\
        \vspace{0.5em}Supplementary Material \\
        \vspace{1.0em}
       % ] %< twocolumn
        }
    }
\maketitlesupplementary

Our supplementary material provides a further extension to our primary findings. We provide additional experimental results in \cref{sec:supp_expr}, delve into the technical details in \cref{sec:supp_method}, and conduct supplementary analysis discussed in \cref{sec:supp_anal}.

\section{Additional Experimental Results}
\label{sec:supp_expr}

\paragraph{Results on SemanticKITTI val.}

We present further quantitative results on the SemanticKITTI \texttt{val} set in \cref{tab:sem_kitti_val} for a more comprehensive comparison. \name{} consistently achieves state-of-the-art performance, aligning with our primary findings.

\input{tab/8_sem_kitti_val}

\section{Extended Technical Details}
\label{sec:supp_method}

\paragraph{Model Size.} 
Our proposed \name{} contains 59.3M parameters (including 16.8M parameters for learnable voxel features), comparable in scale to VoxFormer's 57.9M parameters, and significantly fewer than MonoScene's 149 M. Moreover, \name{} operates at 611.9 GFLOPs, notably fewer than MonoScene's 990.1 GFLOPs. This underscores \name{} maintaining a relatively lightweight yet effective model architecture.

\paragraph{Loss Function.}
We elaborate on the Scene-Class Affinity Loss term $L_{scal}$ in our loss function.

Derived directly from MonoScene~\cite{MonoScene}, $\mathcal{L}_{\text{scal}}$ simultaneously optimizes class-wise derivable (P)recision, (R)ecall and (S)pecificity defined as follows:
\begin{align}
	P_{c}(\hat{p}, p) &= \log\frac{\sum_{i} \hat{p}_{i,c} [ p_i = c ]}{\sum_{i}\hat{p}_{i,c}}, \\
	R_{c}(\hat{p}, p) &= \log\frac{\sum_{i} \hat{p}_{i,c} [ p_i = c ]}{\sum_{i}[ p_i = c ]}, \\
	S_{c}(\hat{p}, p) &= \log\frac{\sum_{i}({1 - \hat{p}_{i,c}}) (1 - [ p_i = c ])}{\sum_{i} (1 - [ p_i = c ])},
\end{align}
where $P_c$ and $R_c$ quantify the performance of similar class $c$ voxels, while $S_c$ measures the performance of dissimilar voxels.

The Scene-Class Affinity Loss $\mathcal{L}_{\text{scal}}$ then maximizes the above class-wise metrics with:
\begin{equation}
	\mathcal{L}_{\text{scal}}(\hat{p}, p) = -\frac{1}{C}\sum_{c = 1}^{C} ({P_c(\hat{p}, p)}  + {R_c(\hat{p}, p)} + {S_c(\hat{p}, p)}).
\end{equation}

\section{Supplementary Analysis and Discussion}
\label{sec:supp_anal}

We summarize the key findings supporting the contributions of our paper:

\paragraph{Instance Semantics.} Symphonies demonstrates superior class IoU scores for instance classes, \eg, buildings, cars, and people, as evidenced in \cref{tab:sem_kitti_test}, \cref{tab:kitti_360_test}, \cref{tab:sem_kitti_val}. Additionally, \cref{fig:vis} illustrates detailed predictions for instances, such as trunks (line 1, 3) and cars (line 1, 4).

\paragraph{Scene Context.} In \cref{fig:vis}, Symphonies exhibits enhanced layouts for buildings and vegetation. Besides, MonoScene's predictions reveal a radial shape indicative of geometric ambiguity, whereas ours maintains a more coherent layout attributed to contextual scene reasoning.
